# Supplementary material for: Examining Large Pre-Trained Language Models for Machine Translation: What You Don't Know About It
Source: arXiv:2209.07417 source file (2022-10-25)
Supplement: Supplementary file 1 [file Appendices.tex]

\label{appendix}
\section*{Appendix A: hLEPOR parameters}
The word level hLEPOR default parameters manually tuned for WMT2013 MT evaluation task across language pairs \cite{han-etal-2013wmt-description,han2013hLEPOR_MTsummit} are displayed as below. Both Python (\url{https://pypi.org/project/hLepor/}) and Perl (\url{https://github.com/lHan87/aaron-project-hlepor}) version codes can be applied to:

On English-to-Czech/Russian (EN=>CS/RU):

\begin{itemize}
    \item \textbf{alpha} = 9.0, 
    \item \textbf{beta} = 1.0,
    \item \textbf{n} = 2,
    \item \textbf{weight_elp} = 2.0,
    \item \textbf{weight_pos} = 1.0,
    \item \textbf{weight_pr} = 7.0.
\end{itemize}

On English-to-German (EN=>DE): 

\begin{itemize}
    \item \textbf{alpha} = 9.0, 
    \item \textbf{beta} = 1.0,
    \item \textbf{n} = 2,
    \item \textbf{weight_elp} = 3.0,
    \item \textbf{weight_pos} = 7.0,
    \item \textbf{weight_pr} = 1.0.
\end{itemize}

On Czech / Spanish / Russian to English (CS/ES/RU =>EN): 

\begin{itemize}
    \item \textbf{alpha} = 1.0
    \item \textbf{beta} = 9.0
    \item \textbf{n} = 2
    \item \textbf{weight_elp} = 2.0
    \item \textbf{weight_pos} = 1.0
    \item \textbf{weight_pr} = 7.0
\end{itemize}

On German/French-to-English (DE/FR=>EN) and English-to-Spanish/French (EN=>ES/FR): 

\begin{itemize}
    \item \textbf{alpha} = 9.0
    \item \textbf{beta} = 1.0
    \item \textbf{n} = 2
    \item \textbf{weight_elp} = 2.0
    \item \textbf{weight_pos} = 1.0
    \item \textbf{weight_pr} = 3.0
\end{itemize}
